# Supplementary material for: Improved Inference of Human Intent by Combining Plan Recognition and Language Feedback
Source: arXiv:2310.02462 source file (2023-10-03)
Supplement: Supplementary file 1 [file appendix.tex]

\section*{Technical Approach}

% So I wouldn't introduce/name the POMDP here but rather cut this little paragraph and move it to where you actually define the DGR-POMDP and start with ``Our problem is..''}

%Imagine a person carrying out a task, such as assembling a piece of furniture or cooking a meal. A person is also typically multitasking  by switching back and forth. There is a hierarchy to these tasks, and the human needs to complete a sequence of instructions to achieve subgoals and complete the subgoals to complete the high-level goal or task, as shown in Fig-\ref{Fig-htn}. 

Given the sensor measurements $O_w$ of the world state $W$, an assistive robot needs to infer the probabilities of the hidden user intent - the human action $\alpha$ that the user is executing and the person's current goal $G$. Partial observability of the latent user intent and noise in the sensor observations impacts accurate inference of $G$, $W$, and $\alpha$  at every sequence of human action.
% A robot must infer the probability distribution of the hidden states $G$, $W$, and $\alpha$
% Because of the noise in $O_w$, the robot will not be able to infer $G$, $W$, and $\alpha$ from the initial world state sensor measurement at every sequence of human action.
We infer the probability distribution of the hidden states $G$, $W$, and $\alpha$ using HTN planning to generate feasible plans for the human-given predefined tasks. We do so by recursively decomposing the composite tasks utilizing a knowledge base and the sensor measurements at each time step to update our belief over human's progress \cite{wang2017hierarchical}.  
% \iinote{st: Can you have one more bit connecting it to the sensor measurements?  The HTN stuff intiializes it from sensor measurements right?}
 \nnote{The
algorithm adopts the hierarchical paradigm in Hierarchical Task Network (HTN) planning
[20], which generates feasible plans for predefined tasks by recursively decomposing composite tasks using a knowledge base. The modeling of ADLs with a HTN framework has
two advantages. First, the hierarchical nature of HTNs enables the algorithm to provide
prompts of different detail levels. Second, the knowledge base allows to set up specific
goals and preferences for the older adults.}
% \iinote{by ....  HTNs are used for planning by default, so give a bit more detail about how it's used for plan recognition here, and cite the previous work.}. 
% However, the inference will be less accurate as the sensors' noisiness increases. 
% The robot 
% A conversational robot can further improve the inference of the hidden states by asking clarification questions. 
With the ability to ask clarification questions, the robot actively improves the inference of the latent states. The human's response - language observations $o_l$ give the agent additional \iinote{noisy} information about their task.
% The humans in response can provide language observations $o_l$ to give more information about their task to the agent. 
We want the robot to decide when to ask questions when, and only when, it gets confused about the belief over human's progress while not bothering the human unnecessarily. We need to balance between information-gathering actions, like asking questions, and goal-inducing actions, such as providing the correct next step. 
Using our D4GR framework, the robot decides when to ask clarification questions and about which human action based on the information gathered from the sensors and language. Our framework avoids asking unnecessary questions and balances between information-gathering actions, like asking questions, and goal-inducing actions, such as providing the correct next step. 
% Our system is able to more accurately infer human intent than these baselines using information gathered from a language without asking unnecessary questions.

\nnote{To achieve a framework for ADL task completion that intelligently asks questions as well as extracts implicit information as the human progresses toward completing the task, we define the Hierarchical Task Network(HTN) based Partially Observable Markov Decision Process, or DGR-MOMDP. Our algorithm uses a MOMDP planner to ask clarifying questions when the robot is confused and determines the desired goal/task that the human is trying to complete by using HTN-based belief update for interpreting natural language input as well as the state of partially observable environment sensors and using MOMDP planner to ask clarifying questions when confused.}

\subsection{POMDP Definition}
\nnote{this part goes in "Background," which is part o Section II - called it Background and Related Work. First, define your problem setting - what are the inputs and outputs of an interactive dialog setting? Then say you're going to model it as a POMDP - define a POMDP. Then talk about all the other systems. For Part III, only talk about the new things due to your work}

We model our \iinote{ask st: active goal recognition} problem as a POMDP~\cite{kaelbling1998planning,shani2013survey,kurniawati2022partially} and solve the POMDP to generate an action policy for the robot. 
Formally, a POMDP is
defined as a tuple ($S,A,T,R,\Omega,O,\gamma
,b_{0}$) where $S$ is a set of
states with $s \in S$; $A$ is a set of actions with $a \in A$; T defines a
transition probability $P( s_t | s_{t-1}, a_{t-1})$; R defines the expected
(immediate, real-valued) reward $r(s_t, a_t)\in {\rm I\!R}$;
$\Omega$ is a set of
observations with $o \in \Omega$; O defines an observation probability
$P(o_t|s_t; a_{t-1})$; $\gamma$ is a geometric discount factor 0 $\leq \gamma 
\leq 1$; and $b_0$ is an initial belief state.

The POMDP operates as follows. At each time step $t$, the world is in some unobserved state $s_t$. Since $s_t$ is not known exactly, a distribution over possible states, named as a belief state $b_t$, is maintained. Thus, $b_{t}(s_t)$ indicates the probability of being in a particular state $s_t$. Based on $b_t$, our robot selects an action $a_t$, receives a reward $r_t$, and transitions to (unobserved) state $s_{t+1}$, where $s_{t+1}$ depends only on $s_t$ and $a_t$. The robot then receives an observation $o_{t+1}$, which is dependent on $s_{t+1}$ and $a_t$. \iinote{talk about the planner}

\nnote{\textbf{MOMDP Formulation for assistive robots:}
POMDPs are used in many approaches for solving decision problems where the environment is noisy and not
perfectly observable. For example, \citet{hoey2010automated} created a decision-making system from a POMDP for a robot helping
dementia patients wash their hands, where the agent must
infer the human's actions and psychological state through
noisy hand and towel tracking. However, this research is limited to step recognition in a single task---washing hands and giving prompts instead of using the language feedback for belief updates. While ours uses language feedback to perform step recognition and do goal recognition for multiple tasks.} 

\subsection{D4GR Formulation} \label{subsec: CD_formulation}
\begin{figure}[t]
    \centering
    \includegraphics[width=0.75\linewidth, keepaspectratio]{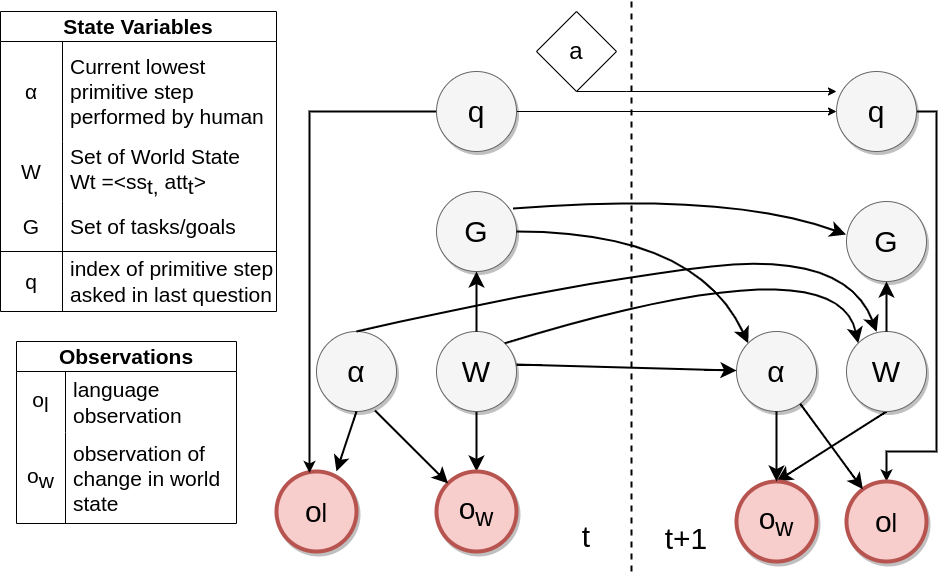}
    \caption{Influence diagram for DGR-POMDP.} 
    % \iinote{Need to change the image}}
    \label{Fig-Influence_diagram_coachdial}
    \end{figure} 
    
% \iinote{is the structure better now?}\stnote{I think you need to define the reward function first before talking about maximizing it. I think you should first define the POMDP and then define the task/goals in the context of the POMDP.  Then the human actions are part of the transition function, and you can define the specific reward function etc.}

We define a novel model, \textbf{D}ialogue \textbf{4}for \textbf{G}oal \textbf{R}ecognition, Partially Observable Markov Decision Process
(D4GR) that enables a robot to maintain a reliable belief state by 
incorporating noisy sensor observations and human language feedback.
% to solve our dialogue assistive goal recognition problem 
% by intelligently selecting when to ask a clarification question \iinote{and provide feedback} based on its belief state. 
\nnote{Solving POMDPs is very challenging; to make progress, we need to define a novel model with specific state representations and independence assumptions that enable us to handle large observation and state space, allowing for efficient inferences. }
For efficient human intent recognition and estimation of optimal action policy, our D4GR 
% must do human plan recognition, but the human actions and 
must be able to handle the large space of the world and language observations 
% that the robot can receive are large. 
% Further, we also want to incorporate human language feedback, but the space of the language observations is also significantly large. 
Our formulation takes advantage of the hierarchical task structure of HTN and makes independent assumptions between state variables set of goals $G$, human action $\alpha$, and world state $W$ to allow for efficient belief update.

% we want to do plan recognition we use the hierarchical structure of HTN and we have large observation space and we make the assumption in the state spxace between goal distribution $G$, human action $\alpha$ and world state $W$ so allow for efficient belief update.

Our D4GR model combines the goal and plan recognition components as described by  \citet{wang2017hierarchical} with the POMDP formalism to allow robots to take action in the environment through dialogue to improve goal recognition. Our D4GR has the following components: ($S,A,T,R,\Omega,O,\gamma
;b_{0}$).
\begin{itemize}
    \item 
    % The state should encode some notion of the instruction step number $i_{t}$ the user’s goal $g_t$, the human's activity $a_{t}$, the state of the world $w_t$, and he intent of the most recent user utterance $u_t$. We will be working on how $a_{t}$ and $w_t$ should look like. To make the model easier we might make the assumption that some variables like $w_t$ are known, therefore making it an Mixed observable MOMDP.
    The state, $s_t \in S$, consists of a tuple of the human mental state, $M_t$, and the world state, $W_t$, along with information needed to track the dialog state.   We represent the human mental state using HTNs. We assume that we have access to the HTN's knowledge graph $TaskNet$  for the tasks, where the root node(s) represent the high-level tasks/goals $G$ that the human can do. The internal nodes of $TaskNet$ are sub-tasks that can be decomposed into leaf nodes depicting primitive human actions $\alpha$. We model the human mental state $M$ represented by $G$ and $\alpha$.
    The $TaskNet$ for our kitchen domain is shown in Fig-\ref{Fig-htn}.

    % as represented an in fig-\ref{Fig-htn}
    For each domain, the $TaskNet$ remains fixed throughout the turns.
    % $G_t$ - the set of goals currently being done by the human as extracted from $TaskNet$ 
    % \kznote{I think the notation $TaskNet$ is not great fo reading. For such a frequent notation, could you use a single letter, possibly with subscript?}
    \nnote{$\alpha_{t}$ the set of lowest primitive steps being done by the human at time $t$ where $\alpha_{i,t} \in \alpha_t$}
    % \kznote{It feels to me quite defensive to talk about the limitation here, when I haven't understood what your algorithm can do.}
     $W_t$ is the world state which is a concatenation of the set of states of the world smart sensors $ss_t$ and the set of the attributes of the objects involved in the task $att_t$ such as dryness of the hand, state of the faucet, etc. $\xi$ is a set of wrong human actions that can lead to sub-optimal or unsuccessful task completion, $q_t$ is the dialog state variable that stores the primitive human action referenced by the robot in its latest clarification question.  Hence the state should be factored into the following components:$s_t=<M_t, \xi, q_t,  W_t,>$
    where $W_t$ = $<ss_t, att_t>$, $M_t=<G_t, \alpha_t>$. 
    Here $G_{t}, \alpha_t, att_t, ss_{t}$ are the hidden variables, while $\xi,;q_{t}$ are the known variables, hence making this a MOMDP \cite{ong2009pomdps}.  The influence diagram can be seen in Fig-\ref{Fig-Influence_diagram_coachdial}.

    \begin{figure}[t]
    \centering
    \includegraphics[width=1\linewidth]{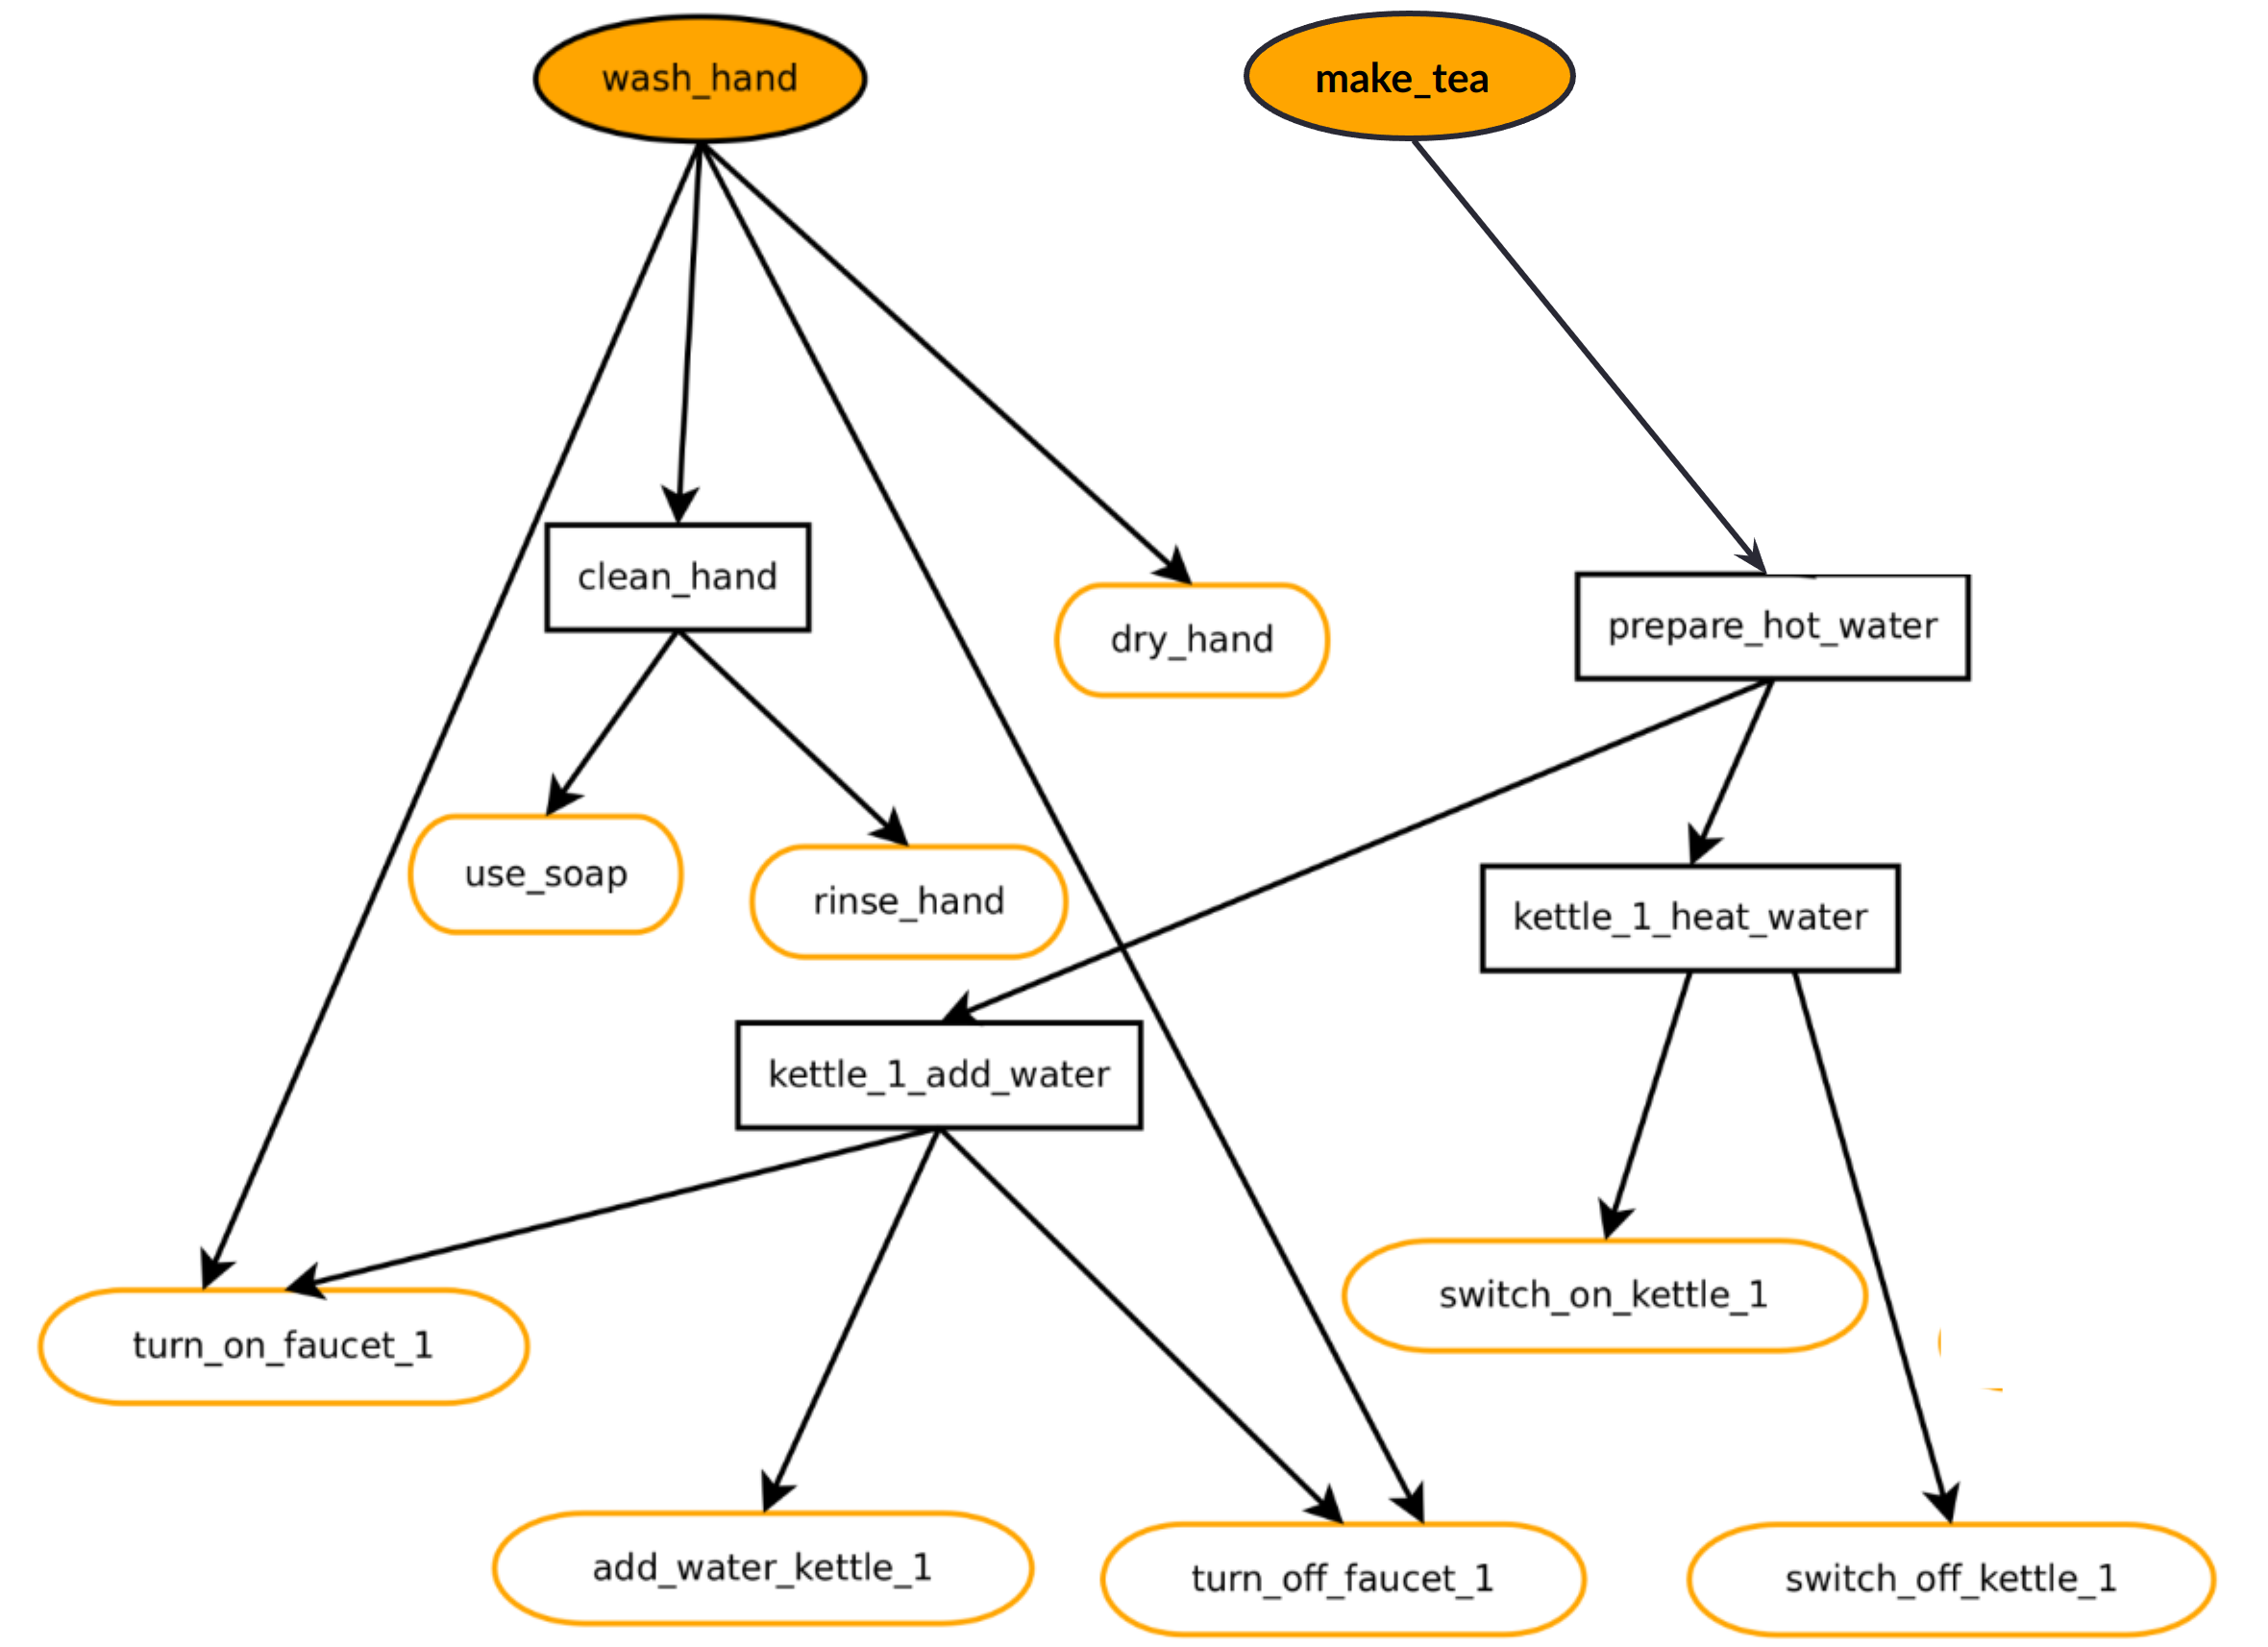}
    \caption{Hierarchical Task Network for three tasks -  washing hands, making tea, and making coffees}
    \label{Fig-htn}
    \end{figure}
    
    \item $A$ includes the actions of the agent. The robot for this research can perform predefined actions only in the language space as follows: $Wait$- do nothing. This only advances the time step,
    $Ask\{argmax(\alpha)\}$
    % {\large{Ask\{argmax($\alpha$)\}}} 
    % \kznote{I haven't seen notation by making the font larger...} 
    - asks a clarification question about $\alpha$, the lowest human primitive actions. When the robot chooses to ask a clarifying question, it asks questions with the following template - ``I believe that you just did action $(\alpha_{i})$, is this correct?''. The argument $i$ is strategically chosen as the primitive action with the highest belief from the state set $\alpha_t$. $inform\_next\_instruction$ informs the agent what human action they should perform at the current timestep based on current belief. This action is chosen based on a fixed policy.
    % $inform\_next\_instruction$ informs the agent what should be the next_instruction based on current belief in the following template. 
    % ``I believe you should be doing action $(\alpha_{i})$''.
    %  action - $inform\_next\_instruction$ informs the agent what should be the next_instruction based on current belief in the following template.
    % ``I believe you should be doing action $(\alpha_{i})$'' where $i$ is the highest belief action from the state set $\alpha_t$
    \iinote{inform\_next\_instruction} 
    % {\large{give_in}}
    % For the purposes of this research, the action that robot can take is carry out dialogue via uttering language sentences or do nothing. 
    % We can divide the action set into two categories. One can change the state of the world such as flip\_world\_state, and the other consists of 
    % only language utterances. Ideal action set for language utterance will include the following actions that can help in safely completing the cooking task: inform\_next\_instruction, negate, affirm, repeat, inform\_doing\_step\_wrong, inform\_state\_world, and bye.
    % \iinote{(thinking of using last question state to know which home appliance are they using)}, tell\_ingredients. 
    % However, we foresee this complicating our transition function formulation, so will work on mitigating it
    \item $\Omega$ consist of the human’s language, $o_l$, and observations about the world state $o_{w}$.  $o_{w}$ includes observations of the world smart sensor's state $ss_t$ and the attributes of the objects involved in the task $att_t$ such as
    $hand\_dry, faucet\_on$, etc. These observations are binary for the states in $W_t$, so the faucet can only be on or off.
    \item $O \equiv P(o_t|s_t; a_{t-1})$ 
    To define the MOMDP, the robot needs a model of $p(o|s)$ $=$ $p(o_l, o_{w}|s)$ to update belief. Most of the complexity of our model is captured in this observation model and belief update defined in the sec-\ref{sec-belief}.
    \item  $T(s,a,s') \equiv p(s_{t+1}|s_t,a_t)$: Our transition function is stochastic.
    %   \stnote{In between each line of math you should have a sentence explaining what it is doing. You dont' need to have every single line, so I might cut equation 3, and then say something like "factored based on assuming that the goal $G$ is conditionally independent of the action given the previous goal or whatever.}
     The overall transition model is shown in Eq-\ref{overall} where we factor our overall mental model $M_t$ into $G_t$ and $\alpha_t$.
    \begin{align*}
    % \centering
    p(s_{t+1}|s_t,a_t) &= p(M_{t+1}, W_{t+1}, q_{t+1}|M_{t}, W_t, q_t, a_t) &\nonumber\\
    & = p(G_{t+1}, \alpha_{t+1}, W_{t+1}, q_{t+1}|G_{t}, \alpha_{t}, W_t, q_t, a_t) &\numberthis\label{overall}\\
    \end{align*}

     % ***********original below*************
    \nnote{\begin{align*}
        & =  p(G_{t+1}, \alpha_{t+1}, W_{t+1}|G_{t}, \alpha_{t}, W_t, a_t) \times p(q_{t+1}|q_{t}, ma_t)&\numberthis\label{factorq} \\ 
    & \hspace{15mm} = p(G_{t+1} | W_{t+1},G_{t}) \times  p(W_{t+1} |  W_{t}, \alpha_{i,t+1})\times &\nonumber\\
    & \qquad p(\alpha_{t+1}|W_{t}, G_{t}) \times p(q_{t+1}|q_{t}, a) &\numberthis
    % & p(G_{t}, NS_t, CS_t, ss_t, att_t, q_t, lo_t, o_{l,t}, o_{w,t} ) &\nonumber
    % &p(CS_t|o_{w,t})  &\nonumber
    \label{eq-state-transition}
    \end{align*}}
\item $R(s,a)$ 
    \nnote{Reward for goal, cost for asking clarification question and time to stay alive}
    We provide a positive reward (5) for asking a clarifying question when the human is doing the wrong lowest primitive step $\xi_i \in \xi$. 
    \nnote{An even larger reward for completing the task successfully (10), within the total number of turns provided to complete the task.} A negative reward (-5) for asking a clarifying question even when the human is doing the correct primitive step or asking a question about a wrong primitive action
    smaller negative rewards for doing nothing (-1). 
    % \iinote{Do these rewards make sense?}.
 \nnote{st: cut, this doesn't make sense with the +5 reward anyway:   The costs of the different actions were initially set to correspond to the number of seconds it would take to complete said action and were tuned from there using both simulated trials and our small pilot study.}

    % They were tuned to result in the highest success rate, regardless of the social feedback paradigm. 
    
    %% \begin{table}[h]
    %% \small
    %% \centering
    
    %% %\stnote{Can you add a column for the formal representation of the query?} \iinote{I had that previously but it was taking too much space so removed it? Will it be okay if we dont have it?}
    %% \stnote{use booktabs, but actually it might be more readable as an equation with large curly braces...like you did in equation 6}
    %% \begin{tabular}{l l l}
    %% % {p{0.4cm}p{3cm}p{3.4cm}} 
    
    %% \toprule
    %%   \bf{a} & \bf{s} & \bf{R} \\
    %% \midrule
    %% wait & * & -1\\
    %% \hline
    %% % Q2 & { "Where was the $attr1$ pink cup"?}  \\
    %% % \hline
    %% Ask(i) & $q_t \in \xi$ & 5\\
    %% \hline
    %%  Ask(i) & $q_t \notin \xi$ & -5\\
    %% \hline
    %% * & $W_t ==$ \text{Desired world state for goal completion} & 10\\
    %% % Q4 & Where is the Sprite bottle \\
    
    %% \bottomrule
    %% % \label{example_queries}
    %% \end{tabular}
    %% % \vspace{-2mm}
    %% % \caption{Query Types, Language Examples \& Formal Representations}
    %% \label{tab:example_queries}
    %% % \vspace{-6mm}
    %% \end{table}
\end{itemize}

\subsection{HTN adaption of Transition Function}\label{sec-transition}

% \stnote{Wrong human actions is overflowing a lot... maybe define $\xi$ outside the equation so it can wrap.}
% \kznote{why put specific numbers here in the equation? Do they really matter for your algorithm?}

We factor in the transition function assuming that at every timestep, the goal, the world state, current primitive human action, , and the last question asked are independent.
    Further, $G_{t+1}$ is conditionally independent of $\alpha_{t+1}$ given the previous goal $G_t$ and world state. 
    \iinote{give reasoning?}
    \begin{align*}
        % & =  p(G_{t+1}, \alpha_{t+1}, W_{t+1}|G_{t}, \alpha_{t}, W_t, a_t) * p(q_{t+1}|q_{t}, ma_t)&\numberthis\label{factorq} \\ 
      p(s_{t+1}|s_t,a_t) = p(G_{t+1} | W_{t+1},G_{t}) \times  p(W_{t+1} |  W_{t}, \alpha_{i,t+1}) \times\\
       p(\alpha_{t+1}|W_{t}, G_{t}) \times p(q_{t+1}|q_{t}, a) &\numberthis
    % & p(G_{t}, NS_t, CS_t, ss_t, att_t, q_t, lo_t, o_{l,t}, o_{w,t} ) &\nonumber
    % &p(CS_t|o_{w,t})  &\nonumber
    \label{eq-state-transition}
    \end{align*}

In the Bayesian network of \cite{wang2017hierarchical}, the world state at the last time point $W_t$ and the goal at time $G_t$ affects the pending human action $\alpha_{t+1}$ - Eq-\ref{eq:currstep-transition}.

\begin{align}
   &p(\alpha_{i,t+1} | w_{i,t}, G_{i,t})&\nonumber\\
%   & = p(\alpha_{i,t+1} | w_{i,t}) &\nonumber\\
& = \begin{cases}
    C \nnote{0.99,0.837},& \text{if } \alpha_{i,t+1} == \text{successor node of HTN}\\
    % & \subset w_{i,t}  \text{ \&}  \\
    %  &  effect(\alpha_{i,t+1}, w_{i,t}) \subset w_{i,t+1} \\
    % &  \\
    1-C \nnote{0.01,0.169},              & \alpha_{i,t+1} \text{ in } \xi
    % \tag{eq:transition}
\end{cases}&
\label{eq:currstep-transition}
\end{align}

$\xi$ is the set of wrong human actions as defined earlier.

The world state at the last time point $W_t$ and the current human action $\alpha_{t+1}$ together contribute to the current world state $W_{t+1}$ - Eq-\ref{eq:world-transition},  and the world state at the current time step $W_{t+1}$ and the goal at time $G_t$ affects the goal at the current time step $G_{t+1}$. Please refer to the cited paper for more details.

\begin{align}
   &p(w_{i,t+1} | w_{i,t}, \alpha_{i,t+1}) = &\nonumber \\
   &\begin{cases}
    0.999,& \text{if } \alpha_{i,t+1}(precondition)\\
    & \subset w_{i,t}  \text{ \&}  \\
     &  effect(\alpha_{i,t+1}, w_{i,t}) \subset w_{i,t+1} \\
    % &  \\
    0.001,              & \text{otherwise}
    % \tag{eq:transition}
\end{cases}&
\label{eq:world-transition}
\end{align} 
    % We also adopt the world transition function - Eq-\ref{eq:world-transition} introduced by \citet{wang2017hierarchical}. 
    % Transition in $w_{t}$ happens as iknowledge graph with subtasks and preconditions that need to be satisfied befroe traversing that subtask branch down 
    % Our state  knowledge graph with subtasks and preconditions that need to be satisfied before traversing that subtask branch down \citet{wang2017hierarchical}. Our transition function is deterministic. 
    
\nnote{We assume that we have access to a knowledge graph for the tasks (HTN) with sub-tasks as nodes that can be decomposed into leaf nodes depicting primitive human actions. HTN for our work is shown in Fig-\ref{Fig-htn}.}

\nnote{\hspace{2mm} The current world state transition -Eq-\ref{eq:world-transition} and human action transition - Eq-\ref{eq:currstep-transition} are rooted in how $TaskNet$ works as a part of HTN. An internal/root node can be decomposed into its children subtasks node if the preconditions are satisfied, leading to stochastic effects in the children nodes.
% before transitioning to the successor state in that particular subtask branch.
This node decomposition process is defined 
% as $\theta$
in \citet{wang2017hierarchical} where the execution of a primitive human action $\alpha_{i,t}$n causes the predefined effects of $\alpha_{i,t}$ to be triggered in the successor state -  $w_{t+1}$
according to the successor node function of HTN predefined \citep{wang2017hierarchical}. The human primitive action transition - $p(\alpha_{i,t+1} | w_{i,t}, G_{i,t+1})$ -- Eq-\ref{eq:currstep-transition} and the constant C are adopted from the extensive experimented test cases introduced in \citet{wang2017hierarchical}.}

We assume that $q_t$ changes deterministically from null to $max\{\alpha_t\}$ after the robot asks a clarifying question. The state variable goal $goal$ is deterministically carried forward to the next time step.
\begin{align}
    &p(q_{i,t+1} | q_{i,t}, a_t) = &\nonumber\\
&\begin{cases}
    1 \text{ for } argmax(\alpha) else 0,& \text{if } a \neq NULL\\
    % &  \\
   1 \text{ for } q_{i,t},else 0              & a_t == NULL
    % \tag{eq:transition}
\end{cases}&
\label{eq:question-transition}
\end{align} 

% \stnote{I would probably define the transition function briefly here in the bullted list, and then make a whole subsection for the factorization after you finish the list.  Just like you did for the observation model.<}

\subsection{Belief Update for Goal Recognition and Planning}\label{sec-belief}
% \stnote{I would make this a subsection of technical approach}
Our belief update performs human intent recognition by maintaining a belief over the hidden human's Mental state $M_t$ represented as goal---$G_{t}$ and the current set of lowest primitive steps executed by the human $\alpha_t$, and also the world state $W_t$.
% The focus of our belief update is 
\nnote{to perform goal and human action recognition and hence estimate the probability distribution of hidden variables: goal setting---$G_{t}$, the current set of lowest primitive steps executed by the human $\alpha_t$, attribute values of the objects involved in the task---$att_t$.} 
% \iinote{Our model also needs to handle stochastic transitions.}
% For this estimation, the observation model plays an important role for updating the belief. 
The actions executed by the human produce an observation of the world state $o_{w}$ specifying the change in the world state $W_t$
%  attribute of the objects and smart home devices involved in the task or change in the state of the smart home devices - $W_t$. 
The user can also produce 
% \iinote{one word language} 
(speech) utterance/feedback $o_{l}$. 
We classify the intent of each sentence into positive or negative feedback using bag of words approach. Our list of the negative responses $r_n$ included \{ ‘no’, ‘nope’, ‘other’, ‘not’ \} and positive responses $r_p$ included the words \{ ‘yes’, ‘yeah’, ‘sure’, ‘yup’ \}.
\iinote{We split $o_{l}$ into two segments: The response utterance $o_{l,r}$ consisting of positive/negative response words, and the base utterance $o_{l,b}$ consisting of all other words. Either of these two strings may be empty $\emptyset$ . To determine which words the user spoke are part of $o_{l,r}$, we compare each word in $o_{l}$ to a list of positive and negative responses. The the negative responses $r_n$ are \{ ‘no’, ‘nope’, ‘other’, ‘not’ \} and positive responses $r_p$ are the words \{ ‘yes’, ‘yeah’, ‘sure’, ‘yup’ \}.}
% Both $o_{w}$ and $o_{l}$ are considered observations.
\iinote{Edit: try $o_w$ as $omega_t$}. 
% Each observation $o \in O$ is a tuple of language $o_{l}$, and world observation $o_{watt}$.
 As a result:
    \begin{equation} \label{o_exp}
    o_t=<o_{l,t}, o_{w,t}>, 
    \end{equation}
where $o_t\in \omega_t$
% \iinote{Edit: add eq - $p(s|o)=$ }
% \iinote{Need to add examples of $o_l$} 
% We split $l$ into two portions: The response utterance lr consisting o positive/negative response words, and the base utterance lb consisting of all other words. Either of these two strings may be empty (). To determine which words the user spoke are part of lr, we compare each word in l to a list of positive and negative responses. The positive responses rp are the words { ‘yes’, ‘yeah’, ‘sure’, ‘yup’ } and the negative responses rn are { ‘no’, ‘nope’, ‘other’, ‘not’ }.

% The belief update a time step $t$, we need to estimate the following:
The belief update equation is as follows:
\nnote{use summation to derive 8 from 6, we should pull language out, rephrase - convert joint distribution into summation and pull language out}

% \begin{align}
% % \begin{align*} 
%     % & (ps_{i,t})_{posterior} = p(ps_{i,t} | o_{w,t}) &\nonumber\\
%     % &= \frac{p( ps_{i,t}, o_{w,t})}{p(o_{w,t})}  \propto p( ps_{i,t}, o_{w,t}) &\nonumber\\
%     % &=\sum_{w_{i,t}} \sum_{w_{i,t-1}}  p( ps_{i,t}, o_{w,t}, w_{i,t}, w_{i,t-1}) &\nonumber\\
%     % &= \sum_{w_{i,t}} \sum_{w_{i,t-1}} p(w_{i,t}| w_{i,t-1}, ps_{i,t}) * p(o_{w,t} | w_{i.t})&\nonumber\\
%     % &  \qquad  \qquad \qquad \qquad \qquad  * p(w_{i,t-1}) * p(ps_{i,t})  &\numberthis \label{eq:posterior_ps_t}
%     & p(s|o) = p(G_{t}, q_{t}, PS_t,  ss_t, att_t, q_t, lo_t|o_{l,t}, o_{w,t} )&\nonumber\\
%     & p(G_{t}, q_{t}, PS_t,  ss_t, att_t, q_t, lo_t|o_{w,t} ) * p(G_{t}, q_{t}, PS_t,  ss_t, att_t, q_t, lo_t|o_{l,t} )           &\nonumber\\
% % \end{align*}
% \end{align}

% \begin{align}
%     & p(s|o) = p(G_{t}, CurrStep_t, ss_t, att_t, q_t|o_{l,t}, o_{w,t} ) &\nonumber\\
%     & = p(G_{t}, NS_t, CS_t, ss_t, att_t, q_t, lo_t, o_{l,t}, o_{w,t} ) &\nonumber
%     &p(CS_t|o_{w,t})  &\nonumber
% \end{align}
% if both $o_{w,t}$ and $o_{l,t} \neq Null$ then posterior of state is as follows:

\begin{align}
    & b'(s_t) = p(s_t|o_{t}, a_{t-1},b_{t-1}) &\nonumber\\
    % & p(s') = n O(o|s',a) \sum_s P(s'|s,a)b(s) &\numberthis
    & \quad\quad = n O(o_{t}, s_{t},a_{t-1}) \sum_s T(s_{t-1},a_{t-1},s_t)b(s_{t-1}). &\numberthis \label{eq-beliefupdate}
\end{align}

% & b'(s') = p(s',o,a, b) &\nonumber\\
% p(s') = n O(z|s',a) \sum_s T(s'|s,a)B(s) &\nonumber\\

% \begin{align}
% & O(s_{t}, a_{t-1},o_{t}) = p(o_t|s_t; a_{t-1}) &\nonumber\\
% & p(o_t, s_t, a_{t-1}) = p(s_t|o_t,a_{t-1}) * p(o_t|a_{t-1}) * p(a_{t-1}) &\nonumber\\
% & p(o_t, s_t, a_{t-1}) = p(o_t|s_t,a_t-1) * p(s_t|a_{t-1}) * p(a_{t-1}) &\nonumber\\
% & p(o_t|s_t,a_{t-1})  = &\nonumber\\
% &\frac{p(s_t|o_t,a_{t-1}) * p(o_t|a_{t-1}) * p(a_{t-1})}{p(s_t|a_{t-1}) * p(a_{t-1})} \nonumber\\
% & p(o_t|s_t,a_{t-1})  = &\nonumber\\
% &\frac{p(s_t|o_t,a_{t-1}) * p(o_t|a_{t-1})}{p(s_t|a_{t-1})} \nonumber\\
% \end{align}
The observation function in Eq-\ref{eq-beliefupdate} can be further expanded and approximated as follows:
\begin{align}
& O(s_{t}, a_{t-1},o_{t}) = p(o_t|s_t; a_{t-1}) &\nonumber\\
% & p(o_t, s_t, a_{t-1}) = p(s_t|o_t,a_{t-1}) * p(o_t|a_{t-1}) * p(a_{t-1}) &\nonumber\\
% & p(o_t, s_t, a_{t-1}) = p(o_t|s_t,a_t-1) * p(s_t|a_{t-1}) * p(a_{t-1}) &\nonumber\\
% & p(o_t|s_t,a_{t-1})  = &\nonumber\\
% &\frac{p(s_t|o_t,a_{t-1}) * p(o_t|a_{t-1}) * p(a_{t-1})}{p(s_t|a_{t-1}) * p(a_{t-1})} \nonumber\\
% & p(o_t|s_t,a_{t-1})  = &\nonumber\\
&\quad\qquad\qquad\quad =\frac{p(s_t|o_t,a_{t-1}) * p(o_t|a_{t-1})}{p(s_t|a_{t-1})} &\nonumber\\
&\quad\qquad\qquad\quad \propto p(s_t|o_t,a_{t-1}) * p(o_t|a_{t-1}). &\numberthis
\end{align}

% \begin{align}
%     & p(s|o) \propto p(G_{t},  CurrStep_t, W_t, q_t, o_{l,t}, o_{w,t} )&\nonumber\\
%     & \propto p(G_{t} | W_t, o_{w,t}) * p( CurrStep_t| o_{l,t}, o_{w,t}) * p(q_t| o_{l,t},o_{w,t}) *  &\nonumber\\
%     & * p(o_{l,t}, o_{w,t}) &\nonumber\\
%     & \propto p(G_t|W_t)*p(W_t|o_{w,t}) * p( CurrStep_t|o_{w,t})* &\nonumber\\
%     & *  p( CurrStep_t| o_{l,t})* p(q_t | o_{l,t})* p(o_{l,t})* p(o_{w,t}) &\nonumber\\
%     & \propto  \underbrace{p(G_t|W_t)*p(W_t|o_{w,t})*p(CurrStep_t| o_{w,t}) * p(o_{w,t})  \rule[-5pt]{0pt}{5pt}}_{\mbox{world belief update}} * &\nonumber\\
%     &\underbrace{p(CurrStep_t, q_t| o_{l,t}) * p(o_{l,t}) \rule[-5pt]{0pt}{5pt}}_{\mbox{language belief update}}&\nonumber
% \end{align}
Overall the derivation of probablity $s_t$ given $o_t$ and $a_{t-1}$ is expanded eq-\ref{eq-observationstateupdate} to Eq-\ref{eq-factormodels}. 
% in Eq-\ref{eq-observationstateupdate}, we perform derivation through     
% \stnote{Isn't this conditinally independent given the state? Since they are the observations, they should be completely determined given the observation.  Also I think you don't need to make an experimental argument.  First you can't just say ``we ran experiments'' without giving the experiments.  So we should have a section in the evaluation for that if we want to make that argument.  But really I think ti's reasonable to assume that they are independent given the state (because you know the full state so then the two parts of the observation are determined based on the state not each other)... } 
\iinote{st: You again don't need to show every single step.  I like to write it all out to vet the math; once it's vetted you can skip steps when explaining it.}
\nnote{\begin{align}
    & p(s_t|o_t, a_{t-1})&\numberthis\label{eq-observationstateupdate}\\
    & \propto p(G_{t},  \alpha_t, W_t, q_t, o_{l,t}, o_{w,t}, a_{t-1} )&\label{eq-jointdist}\numberthis\\
    & \propto p(G_{t},  \alpha_t, W_t, q_t | o_{l,t}, o_{w,t}, a_{t-1}) *  p(o_{l,t}, o_{w,t}, a_{t-1}) &\label{eq-factor1}\numberthis\\
    & \propto p(G_{t}, W_t| o_{l,t}, o_{w,t}, a_{t-1}) * p(q_t | o_{l,t}, o_{w,t}, a_{t-1})&\nonumber\\
    &  \qquad p(\alpha_t | o_{l,t}, o_{w,t}, a_{t-1}) * p(o_{l,t}, o_{w,t}, a_{t-1}). &\label{eq-factor2}\numberthis
\end{align}}

\begin{align}
    & p(s_t|o_t, a_{t-1})&\numberthis\label{eq-observationstateupdate}\\
    % & \propto p(G_{t},  \alpha_t, W_t, q_t, o_{l,t}, o_{w,t}, a_{t-1} )&\label{eq-jointdist}\numberthis\\
    & = p(G_{t},  \alpha_t, W_t, q_t | o_{l,t}, o_{w,t}, a_{t-1}) *  p(o_{l,t}, o_{w,t}, a_{t-1}) &\label{eq-factor1}
    % & \propto p(G_{t}, W_t| o_{l,t}, o_{w,t}, a_{t-1}) * p(q_t | o_{l,t}, o_{w,t}, a_{t-1})&\nonumber\\
    % &  \qquad p(\alpha_t | o_{l,t}, o_{w,t}, a_{t-1}) * p(o_{l,t}, o_{w,t}, a_{t-1}) &\label{eq-factor2}\numberthis
\end{align}

% The joint distribution in Eq-\ref{eq-jointdist} can be factorized into

Our observation function can be factored to  Eq-\ref{eq-independence_ass1} because of our assumption that human action referenced in the last question asked---$q$, current human action- $\alpha$, and goal \& world state---$(G, W)$ are independent of each other given the observation and the goal $G$, the human action $\alpha$ at the current timestep are independent of the robot's action at the previous timestep resulting in Eq-\ref{eq-independence_ass1}.

\begin{align}
     & \propto p(G_{t}, W_t| o_{l,t}, o_{w,t}) * p(q_t | o_{l,t}, o_{w,t}, a_{t-1})&\nonumber\\
     & \qquad p(\alpha_t | o_{l,t}, o_{w,t}) * p(o_{l,t}, o_{w,t}, a_{t-1}) &\numberthis\label{eq-independence_ass1} 
\end{align}

Further, Fig-\ref{Fig-Influence_diagram_coachdial} shows that world observation $o_{w,t}$ provides us information only about the  $W$ and $\alpha$ while the language observation is relevant to the human action $\alpha$, the last question asked $q_t$, consequently affecting the goal. 
% Further, both the observations are independent of the previous action resulting in Eq-\ref{eq-independence_ass2}. 
% \begin{align}
%      & \propto p(G_{t}, W_t| o_{w,t}) * p(q_t | o_{l,t}, a_{t-1})&\nonumber\\
%      & \qquad p(\alpha_t | o_{l,t}, o_{w,t}) * p(o_{l,t}, o_{w,t}, a_{t-1}) &\numberthis\label{eq-independence_ass2}
% \end{align}
Goal $G$ and $W$ given $o_{w,t}$ can be factorized into
Eq-\ref{eq-factormodels} that can be grouped together into  world observation model and language observation model in Eq-\ref{eq-factormodels}.In the derived Eq-\ref{eq-factormodels}, the language and world observational components can be factored based on the assumption that the states are conditionally independent given the observation.

% because  $o_{w,t}$ depends on the world state $W_t$ which in turn affects the goal $G_t$. 
% Eq-\ref{eq-independence_ass3} because  $o_{w,t}$ depends on the world state $W_t$ which in turn affects the goal $G_t$.  Eq-\ref{eq-independence_ass3} can be grouped together into  world observation model and language observation model in Eq-\ref{eq-factormodels}. In the derived Eq-\ref{eq-factormodels}, the language and world observational components can be factored based on the assumption that the states are conditionally independent given the observation. 
% \footnote{We ran extensive experiments that showed making this conditional independence does not adversely impact the performance of our dialogue planner}.

\begin{align}
    % & \propto p(G_t|W_t)* p(W_t|o_{w,t}) *  p(q_t | o_{l,t})* p(q_t | a_{t-1}) &\nonumber\\
    % & *  p( \alpha_t|o_{w,t})* p( \alpha_t| o_{l,t})* p(o_{l,t})* p(o_{w,t}) &\numberthis\label{eq-independence_ass3}\\
    & \propto  \underbrace{p(G_t|W_t)*p(W_t|o_{w,t})*p(\alpha_t| o_{w,t}) * p(o_{w,t})  \rule[-5pt]{0pt}{5pt}}_{\mbox{world observational model}} * &\nonumber\\
    &\underbrace{p(\alpha_t, q_t| o_{l,t}) * p(o_{l,t}) * p(q_t | a_{t-1}) \rule[-5pt]{0pt}{5pt}}_{\mbox{language observational model}}&\label{eq-factormodels}\numberthis
\end{align}

\iinote{dealt with action in eq-\ref{eq-independence_ass1}?}\iinote{dealt with action in eq-\ref{eq-factormodels}?}
For the world belief update, the components --- $p(G_t|W_t)$, $p(W_t|o_{w,t})$ and $p(\alpha_{t}| o_{w,t})$  are derived from the work of \citet{wang2017hierarchical}.

% For detailed explanation of the equation goal inference update - $p(G_t|W_t)$ please refer to the cited paper. 
% The latter two equations 

\begin{align}
    %  &p(\alpha_{t}| o_{w,t})
    %  \propto \sum_{w_{t-1} \in W_{t-1}} \sum_{w_{t} \in W_{t}} p(\alpha_t, &\nonumber\\
    %  & \quad\quad\quad\quad\quad\qquad\qquad\qquad \quad\qquad\qquad\quad o_{w,t}, w_{t-1}, w_t)& \label{eq-currstep}\numberthis
     &p(\alpha_{t}| o_{w,t})
     \propto \sum_{w_{t-1} \in W_{t-1}} \sum_{w_{t} \in W_{t}} p(\alpha_t,  o_{w,t}, w_{t-1}, w_t)& \label{eq-currstep}\numberthis
\end{align}

\begin{align}
    & p(W_t|o_{w,t})=\sum_{w_{t-1} \in W_{t-1}}  \sum_{\alpha_{i,t} \in \alpha_{t}} p(\alpha_{i,t}, o_{w,t}, w_{t-1}, w_t) & \label{eq-world}\numberthis
\end{align}

Both step recognition result $p(\alpha_{t}| o_{w,t})$ and world state update $p(W_t|o_{w,t})$ adopt Bayesian update as described below in Eq-\ref{eq-currstep} \nnote{fix this equation} and Eq-\ref{eq-world}. The proposed algorithm for goal recognition in $p(G_t|W_t)$ in \citet{wang2017hierarchical} relies on explanations $expla$. $p(G_t|W_t)$ reasons with explanations in $ExplaSet$ that explain the observations so far. Further details can be found in \citep{wang2017hierarchical}. $p(o_{w,t})$ depends on sample sensor probability of the detectors. We adopt the same noise model for the sensor as described by \citet{wang2017hierarchical}. If $o_{w,t} == Null$ then $o_{w,t}$ does not trigger the world belief update. 
\iinote{The probability of goal $p(G_t|W_t)$ is the sum of probabilities of $expla \in ExplaSet$  whose $startGoal$ contains $g_{i,t}\in G_t $.}

\nnote{Appendix: Both step recognition result $PS'_{t,posterior}$ 
% updated after handling the wrong step as described below
and $W_{t, posterior}$ 
\iinote{do I need to show more explicit connection between $att_{i,t}$ and $W_{t}$  }
which is updated according to Eq-\ref{eq:wt} are fed as input to update $ExplaSet$. This updated $ExplaSet$ is used to calculate Posterior of $G_t$. 
% Fig-\ref{fig:ExplaSet Update} shows the procedure to update the ExplaSet. 
Given a step $ps_{i,t} \in PS'_{t,posterior}$, each explanation $expla{i,t} \in ExplaSet_{t}$ will be updated to several new ones, which are stored in $ExplaSet_{posterior}$.
This includes two procedures: recognition and decomposition. Details can be found in \cite{wang2017hierarchical}. The important equation to remember is that the  
%  The recognitionprocedure adopts a new $goalNet_{t} \in forest_{t} \subset expla_{t}$ to represent the new ongoing status of the corresponding goal and computes 
probability of new explanation is computed using Equation-\ref{eq:ex}
\begin{align}
    &p(new_{expla})= p((ps_{i,t})_{posterior}) * goalNet(expandProb) & \nonumber\\
    &\qquad \qquad \qquad *p(expla) \label{eq:ex}& 
\end{align}
The probability of goal $g_{i,t}$ in $G_t$ is the sum of probabilities of $expla \in ExplaSet$  whose $startGoal$ contains $g_{i,t}$. The probability of $ (ps_{i,t})_{posterior} \in PS_t$ is updated to be the sum of probabilities of explanations $expla \in ExplaSet$ whose $forest$ contains a node standing for $ps_{i,t}$ with completeness being false while readiness being true.
}

\nnote{Prior state probability is calculated as follows:
\begin{align}
    & \text{ prior } = p(s_t) &\nonumber\\
    & \text{ where }  s_t =  <G_{t}, CurrStep_t,  ss_t, att_t, q_t> &\nonumber\\
    % & \propto p(s_t, s_{t-1}, a_{t-1})  &\nonumber\\
    &\propto \sum_{a_{t-1} \in A_{t-1}} \sum_{s_{t-1} \in S_{t-1}} p(s_t, s_{t-1}, a_{t-1})  &\nonumber\\
     &\propto \sum_{a_{t-1} \in A_{t-1}} \sum_{s_{t-1} \in S_{t-1}} p(s_t| s_{t-1}, a_{t-1}) * p(s_{t-1}) * p(a_{t-1}))  &\numberthis
    % & p(G_{t}, CurrStep_t,  ss_t, att_t, q_t) &\nonumber\\
    % & = \sum_{a \in A} \sum_{}  p(G_{t}, CurrStep_t,  ss_t, att_t, q_t| )&
    % & = p(G_t | ss_t, att_t)*p(ss_t, att_t | CurrStep_t, W_{t-1})&\nonumber\\
    % &\qquad *p(CurrStep_t|G_{t-1}, W_{1-1})*p(q_t| q_{t-1})&
\end{align}}

\iinote{This assumption of cooperation is what allows the robot to gather more information from the speaker's utterance, making the interaction quicker and more efficient. }
Derivation of the language observational model is shown in Eq-\ref{eq-langmodel} \iinote{alpha?}.

\stnote{So with all the success of deep models, one criticism is ``why not just use GPT-3?''  I think the answer is that GPT is not grounded:  it is not clear how to connect the information from GPT to the sensor abstraction.  But in this model you are explicitly connecting the sensor information to semantics with the POMDP, that's what the transition model is doing.    But then I think you could incorporate GPT-3 or LLMs by using them to define this probability with the right prompt, and then getting a confidence score.  I think you should at minimum say that's a thing you could do, but you didn't do it because it's not the focus of this paper.  This would let you interpret more open-ended language and/or ask more open-ended questions.}

\begin{align}
    & \textit{language observational model = } p(\alpha_t, q_t| o_{l,t}) * p(o_{l,t})&\nonumber\\
    &\qquad\qquad\qquad\qquad\qquad\qquad\propto p(\alpha_t, q_t, o_{l,t})&\nonumber\\
    &\qquad\qquad\qquad\qquad\qquad\qquad\propto p(o_{l,t} | \alpha_t, q_t)*p(\alpha_t, q_t) &\nonumber\\
    % & \propto p(\alpha_t, o_{l,t})&\nonumber\\
    & \qquad\qquad\qquad\qquad\qquad\qquad\propto p(o_{l,t} | \alpha_t, q_t) &\label{eq-langmodel}\numberthis
\end{align}

We can estimate the effect of the language observation $o_l$ on $\alpha$ and $q$ by calculating the $p(o_{l,t} | \alpha_t, q_t)$. To calculate $p(o_{l,t} | \alpha_t, q_t)$, we consider three possibilities for the state: $\alpha_t = q_t$, $\alpha_t \neq q_t$ and $\alpha = Null$.
If $\alpha_t = q_t$,  then it is very likely that the user will respond with a positive/confirmation feedback. 
% To calculate p(u|s), we must consider three possibilities.
If $\alpha_t \neq q_t$, then the opposite is true. If $q_t = Null$, then no question has been asked, so both types of responses are equally likely. The
mathematical representation of $p(o_{l,t} | \alpha_t, q_t)$. is governed by the
following conditional probability table:
% for the state: ir = id, ir 6= id, and ir = null. If
% ir = id, then it is very likely that the user will respond
% with a positive utterance, and very unlikely that they will
% respond with a negative utterance. If ir 6= id, then the
% opposite is true. If ir = null, then no question has been
% asked, so both types of responses are equally likely. The
% mathematical representation of p (u | s) is governed by the
% following conditional probability table:

\begin{table}[h]
    \small
    \centering
    \begin{tabular}{l c c}
    \toprule
      & $p(o_{l,t} = Yes)$& $p(o_{l,t} = No)$ \\
    \midrule
    $\alpha_{t} = q_t$ & $0.99$ & $0.01$\\
    $\alpha_{t} \neq q_t$ & $0.01$ & $0.99$\\
    $q_{t} = Null$ & $0.5$ & $0.5$\\
    % Sensor Data Size (GB) & 10.53 & $1.43$\\
    \bottomrule
    \end{tabular}
    % \vspace{-3mm}
    \caption{$p( o_{l,t+1}| \alpha_{t}, q_{t})$}
    \vspace{-10mm}
    \label{tab:o==Yes}
% \vspace{-3mm}
\end{table}

At each time step as the human performs action, we use a MOMDP by using an approximate solver, POUCT \cite{silver2010monte} to approximate the optimal policy for robot communication with the human. We then use our observational model to update the our belief of human's mental state $M = G,\alpha$.

\nnote{
For language feedback, $p(G | G, q, o_l)$
\begin{align}
    & \text{language belief update = } p(CurrStep_t, q_t| o_{l,t})&\nonumber\\
    % & \propto p(CurrStep_t, o_{l,t})&\nonumber\\
    & \propto p(o_{l,t} | CurrStep_t, q_t, ) &\nonumber\\
\end{align}
\begin{align}
    & p(o_{l,t}  | q_{i,t}, currstep_{t}) = &\nonumber\\
& \begin{cases}
    p(o_{l,t}) * p(o_{l,t}  | q_{i,t}, currstep_{i,t}) ,& \text{if } o_{l,t} \neq NULL \\
    % &  \\
    1 - o_{l,t} ,              & \text{otherwise}
    % \tag{eq:transition}
\end{cases} &
% \label{eq:world-transition}
\end{align}
}
\nnote{
\begin{align}
    & p(s|o) \propto p(G_{t},  CurrStep_t, W_t, q_t, o_{l,t}, o_{w,t} )&\nonumber\\
    & \sum_{w_{t-1} \in W_{t-1}} \sum_{currstep_{t} \in CurrStep_{t}} (p(CurrStep_t| o_{w,t})) &\nonumber\\
    &\propto \sum_{w_{t-1} \in W_{t-1}} \sum_{currstep_{t} \in CurrStep_{t}} \Bigg ( \sum_{w_{t-1} \in W_{t-1}}  \sum_{w_{t} \in W_{t}}   &\nonumber\\
    &p(G_{t},  currstep_t, w_t, q_t, o_{l,t}, o_{w,t}, w_t, w_{t-1}) \Bigg ) &\nonumber\\
    & p(G_{t},  CurrStep_t, w_t, q_t, o_{l,t}, w_{t-1}, o_{w,t} ) &\nonumber\\
    & \propto\sum_{w_{t-1} \in W_{t-1}}  \sum_{w_{t} \in W_{t}} &\nonumber\\
    & p(w_t| currstep_{t}, w_{t-1}) * p(o_{w,t} | w_t) * p(w_{t-1}) * p(currstep_{t}) &\nonumber\\
    &* p(G_{t}, q_t, w_t, o_{l,t}, o_{w,t})&\nonumber\\
    &  \propto p(G_{t},  CurrStep_t, ss_t, att_t, q_t, o_{l,t}, o_{w,t} )&\nonumber\\
    & = \frac{\splitfrac{ \underbrace{p(o_{l,t}, o_{w,t} | G_{t}, CurrStep_t, ss_t, att_t, q_t) \rule[-5pt]{0pt}{5pt}}_{\mbox{observational model}} } {* p( G_{t}, NS_t, CurrStep_t,ss_t, att_t, q_t)}}{p(o_{l,t}, o_{w,t})} & \numberthis
    % \underbrace{\frac{\hbar\omega_{\mathrm{a}}}{2}\sigma_3                      \rule[-12pt]{0pt}{5pt}}_{\mbox{atom}}
\end{align}
\begin{align}
    & p(s|o) = p(G_{t},  CurrStep_t, ss_t, att_t, q_t|o_{l,t}, o_{w,t} )&\nonumber\\
    & = \frac{\splitfrac{ \underbrace{p(o_{l,t}, o_{w,t} | G_{t}, CurrStep_t, ss_t, att_t, q_t) \rule[-5pt]{0pt}{5pt}}_{\mbox{observational model}} } {* p( G_{t}, NS_t, CurrStep_t,ss_t, att_t, q_t)}}{p(o_{l,t}, o_{w,t})} & \numberthis
    % \underbrace{\frac{\hbar\omega_{\mathrm{a}}}{2}\sigma_3                      \rule[-12pt]{0pt}{5pt}}_{\mbox{atom}}
\end{align}
\begin{align}
    &\text{observational model} = &\\
    &p(o_{l,t}, o_{w,t} | G_{t}, q_{t}, CurrStep_t,  ss_t, att_t) &\nonumber\\
    & = \underbrace{p(o_{l,t}| G_{t},CurrStep_t,  ss_t, att_t, q_t, lo_t) \rule[-5pt]{0pt}{5pt}}_{\mbox{language observational model}} * &\nonumber\\
    & \underbrace{p(o_{w,t} | G_{t}, CurrStep_t,  ss_t, att_t, q_t, lo_t) \rule[-5pt]{0pt}{5pt}}_{\mbox{world observational model}}  &\numberthis
\end{align}
\bknote{Question: Is the following step okay?}\\
if $o_{w,t} \neq Null$ then posterior of state is as follows:
\begin{align}
    & \text{world observational model = } &\\
    & p(o_{w,t} | G_{t}, CurrStep_t,  ss_t, att_t, q_t)&\nonumber\\
    & = \frac{\splitfrac{ \underbrace{p(G_{t}, CurrStep_t,  ss_t, att_t, q_t|o_{w,t}) \rule[-5pt]{0pt}{5pt}}_{\mbox{state posterior}} } {* p(G_{t}, CurrStep_t,  ss_t, att_t, q_t)}}{p(o_{w,t})}&\numberthis
    % & = \frac{\splitfrac{p(G_{t}, CurrStep_t,  ss_t, att_t, q_t|o_{w,t})} {* p(G_{t}, CurrStep_t,  ss_t, att_t, q_t)}}{p(o_{w,t})}&\numberthis
    % \underbrace{\frac{\hbar\omega_{\mathrm{a}}}{2}\sigma_3                      }
\end{align}
\bknote{does the following makes sense?, what to do with $G_t$ and its relation to $o_t$ and parent of ow is W}
\begin{align}
    & \text{state posterior} = &\nonumber\\
    &p(G_{t}, CurrStep_t, ss_t, att_t, q_t|o_{w,t})&\nonumber\\
    & \propto p(G_{t}, CurrStep_t, ss_t, att_t, q_t, o_{w,t})  &\nonumber\\
    & \propto P(CurrStep_t|o_{w,t}) * P(att_{t}|o_{w,t}) * p(G_{t} | o_{w,t}) &\nonumber\\
    &* P(ss_t|o_{w,t})* P(q_t|o_{w,t}) &\nonumber\\
    & \propto P(CurrStep_t|o_{w,t}) * P(att_{i,t}|o_{w,t}) * p(G_{t} | o_{w,t}) 
    \label{eq-posterior_state_world}
\end{align}
The terms in Eq-\ref{eq-posterior_state_world} is calculated as described by \cite{wang2017hierarchical}. It is also mentioned in our appendix section.
\bknote{Question -  Ask Eric does this makes sense?}
if $o_{w,t} == Null$ then posterior of state is as follows:
\begin{align}
    &p(o_{w,t} | G_{t}, q_{t}, CurrStep_t,  ss_t, att_t)&\nonumber\\
    &=1-p(o_{w,t})& 
\end{align}
where $p(o_{w,t}) = 0.95$ \\
}

\nnote{\appendix
The belief update a time step $t$, given $o_{w,t}$ is as follows. Posterior of $ps_{i,t} \in PS_t$ is calculated by the method adopted in HTN using Equation-\ref{eq:posterior_ps_t}. 
\begin{align}
% \begin{align*} 
    & (ps_{i,t})_{posterior} = p(ps_{i,t} | o_{w,t}) &\nonumber\\
    &= \frac{p( ps_{i,t}, o_{w,t})}{p(o_{w,t})}  \propto p( ps_{i,t}, o_{w,t}) &\nonumber\\
    &=\sum_{w_{i,t}} \sum_{w_{i,t-1}}  p( ps_{i,t}, o_{w,t}, w_{i,t}, w_{i,t-1}) &\nonumber\\
    &= \sum_{w_{i,t}} \sum_{w_{i,t-1}} p(w_{i,t}| w_{i,t-1}, ps_{i,t}) * p(o_{w,t} | w_{i.t})&\nonumber\\
    &  \qquad  \qquad \qquad \qquad \qquad  * p(w_{i,t-1}) * p(ps_{i,t})  &\numberthis \label{eq:posterior_ps_t}
% \end{align*}
\end{align}

$ss_t \subset W_t$ is fully observable and Posterior of $att_{i,t} \in att_t \subset W_t$ is dependant on $(ps_{i,t})_{posterior}$ and is calculated as follows:
% (ps_{i,t})_{posterior} 

% \begin{align*}
\begin{align}
    & (att_{i,t})_{posterior} = p(att_{i,t} | o_{w,t}) &\nonumber\\
    &=\sum_{att_{i,t-1}} \sum_{ps'_{i,t} \in (ps_{i,t})_{posterior}}  p(att_{i,t}| att_{i,t-1}, ps'_{i,t}) * p(o_{w,t} | att_{i,t}) &\nonumber\\
    & \qquad  \qquad \qquad \qquad \qquad * p(w_{i,t-1}) * p(ps'_{i,t}) &\label{eq:wt} 
\end{align}
}
% \end{align*}

% \textbf{Explanation Set Update \& Wrong Step Handling}:

% Based on $(ps_{i,t})_{posterior}$ and rollouts of planning algorithm, the agent will take an action $a_t \in A$.  At step $t+1$, $ (ps_{i,t+1}) = (ps_{i,t})_{posterior}$, $lq_{t+1}$ is transitioned deterministically, 
